# Supplementary material for: Direct visualization of three-dimensional shape of skyrmion strings in a noncentrosymmetric magnet
Source: arXiv:2102.05556 ancillary file (2021-02-10)
Supplement: Supplementary file 1 [file Supplementary_Video_Legends.pdf]

# Supplementary Video Legends: Direct visualization of three-dimensional shape of skyrmion strings in a noncentrosymmetric magnet

S. Seki[1,2,3,4,*], M. Suzuki[5,*], M. Ishibashi[6], R. Takagi[1,2,3], N. D. Khanh[3], Y. Shiota[6], W. Koshibae[3], Y. Tokura[1,3,7], T. Ono[6,8,*]

[1] *Department of Applied Physics, University of Tokyo, Tokyo 113-8656, Japan,*

[2] *Institute of Engineering Innovation, University of Tokyo, Tokyo 113-8656, Japan,*

[3] *RIKEN Center for Emergent Matter Science (CEMS), Wako 351-0198, Japan,*

[4] *PRESTO, Japan Science and Technology Agency (JST), Kawaguchi 332-0012, Japan,*

[5] *Japan Synchrotron Radiation Research Institute, Sayo 679-5198, Japan,*

[6] *Institute for Chemical Research, Kyoto University, Uji 611-0011, Japan,*

[7] *Tokyo College, University of Tokyo, Tokyo 113-8656, Japan,*

[8] *Center for Spintronics Research Network, Graduate School of Engineering Science, Osaka University, Toyonaka 560-853, Japan*

## I. SUPPLEMENTARY VIDEO 1

A series of XMCD images taken from various angles $-90^\circ \leq \theta \leq 90^\circ$ with $5^\circ$ steps. The images taken at selected $\theta$ value are shown in Fig. 3.

## II. SUPPLEMENTARY VIDEO 2

$360^\circ$ view of the experimentally reconstructed $m^c(\mathbf{r})$ profiles. The definition of background color is the same as Fig. 4b and c in the main text.

## III. SUPPLEMENTARY VIDEO 3

Slice animation of experimentally reconstructed $m^c(\mathbf{r})$ profiles, where the slice position is changed as a function of time. The selected slice images are shown in Fig. 4b and c in the main text.
